# Supplementary material for: Learning Hierarchical Polynomials of Multiple Nonlinear Features with Three-Layer Networks
Source: arXiv:2411.17201 source file (2024-11-26)
Supplement: Supplementary file 1 [file Appendix_Experiments.tex]

\clearpage
\section{Omitted Experimental Settings and Results}\label{appendix::experiments}
